# Supplementary material for: Probing context-dependent errors in quantum processors
Source: arXiv:1810.05651 ancillary file (2018-10-12)
Supplement: Supplementary file 1 [file Fig2.ipynb.pdf]

```
In [1]: from __future__ import division, print_function

import pygsti
import numpy as np
import scipy
from scipy import stats
from matplotlib import pyplot as plt
%matplotlib inline
import seaborn
seaborn.set()
```

```
/Users/kmrudin/pyGSTi/packages/pygsti/tools/matrixtools.py:23: UserWarning: Could not import Cython extension - falling back to slower pure-python routines
  _warnings.warn("Could not import Cython extension - falling back to slower pure-python routines")
```

## Generating the data

```
In [2]: # Imports a gate set consisting of X and Y rotations by pi/2
from pygsti.construction import std1Q_XY
# Creates the long-sequence GST circuits
germs = std1Q_XY.germs
fiducials = std1Q_XY.fiducials
max_lengths = [1,2,4,8,16,32,64,128,256]
gate_sequences = pygsti.construction.make_lsgst_experiment_list(std1Q_XY.germs, max_lengths)
print("The total number of circuits is {}".format(len(gate_sequences)))
```

The total number of circuits is 1405

```
In [3]: #Let's make our underlying gate set have a little bit of random unitary noise
#Choose if you want to use the same random base gate set used to generate the data
#or if you want to generate your own random base gate set.

load_or_generate_gs = 'load'
#load_or_generate_gs = 'generate'

if load_or_generate_gs == 'load':
    gs_exp_0 = pygsti.io.load_gateset('Simulated_data/base_gate_set.txt')

elif load_or_generate_gs == 'generate':
    gs_exp_0 = std1Q_XY.gs_target.copy()
    gs_exp_0 = gs_exp_0.randomize_with_unitary(.01, seed=0)
```

```
In [4]: np.random.seed(0)
np.random.randn()
```

Out[4]: 1.764052345967664

```
In [5]: #Now we make a list of gate sets, each with an additional  $10^{-3}$  radians of c

gs_linear_list = []
angle_scale = 1e-3
for i in range(5):
    angle = angle_scale*i
    new_gs = gs_exp_0.copy()
    new_gs['Gx'].rotate((angle,0,0))
    new_gs['Gy'].rotate((0,angle,0))
    gs_linear_list.append(new_gs)
```

```
In [6]: N=100
num_passes = 5
```

```
In [7]: ds_linear_list = []
```

```
In [8]: #Now we generate or load datasets, one for each gate set.
#If 'generate' is selected, then the data gets regenerated.
#If 'load' is selected, then the data presented in the paper is loaded
#(which might not be the same as the regenerated data, due to random sampling)

load_or_generate_ds = 'load'
#load_or_generate_ds = 'generate'

if load_or_generate_ds == 'load':
    for i in range(num_passes):
        print("Loading data for pass {}".format(i+1))
        ds_linear = pygsti.io.load_dataset('Simulated_data/ds_linear_'+str(i+1))
        ds_linear_list.append(ds_linear)

if load_or_generate_ds == 'generate':
    for i in range(num_passes):
        print("Generating data for pass {}".format(i+1))
        ds_linear = pygsti.construction.generate_fake_data(gs_linear_list[i])
        ds_linear_list.append(ds_linear)
```

```
Generating data for pass 1
Generating data for pass 2
Generating data for pass 3
Generating data for pass 4
Generating data for pass 5
```

## Data analysis

```
In [9]: # We fix the global significance of the hypothesis testing to be 5%.
global_significance_level = 0.05
```

```
In [10]: #We perform 11 "top level" tests- 10 pairwise comparisons, and 1 comparison
number_of_toplevel_tests = 10 + 1
corrected_significance_level = global_significance_level/number_of_toplevel_
print(corrected_significance_level)
```

```
0.004545454545454546
```

```
In [11]: comparators_dict = {}
```

```
In [12]: print("-----")
print("----- Jointly comparing all passes (comparing {} contexts) -----")
print("-----")
alldata = [ds_linear_list[i] for i in range(num_passes)]
comparators_dict['all'] = pygsti.objects.DataComparator(alldata)
comparators_dict['all'].implement(significance=corrected_significance_level)
```

```
-----
----- Jointly comparing all passes (comparing 5 contexts) -----
-----
```

The datasets are INCONSISTENT at 0.4545454545454546% significance.

Details:

- Using the composite log-likelihood ratio test, the significance of the inconsistency between datasets is 21.76812957323158 standard deviations.
- The number of sequences with data that is inconsistent is 21

```
In [13]: num_passes = 5
         for i in range(num_passes):
             for j in range(i+1, num_passes):
                 print("-----")
                 print("--- Comparing pass {} to pass {} (comparing 2 contexts) ---")
                 print("-----\n")
                 comparators_dict[i,j] = pygsti.objects.DataComparator([ds_linear_list[i], ds_linear_list[j]])
                 comparators_dict[i,j].implement(significance=corrected_significance)
                 print('')
```

```
-----
--- Comparing pass 1 to pass 2 (comparing 2 contexts) ---
-----
```

Statistical hypothesis tests did NOT find inconsistency between the datasets at 0.4545454545454546% significance.

```
-----
--- Comparing pass 1 to pass 3 (comparing 2 contexts) ---
-----
```

The datasets are INCONSISTENT at 0.4545454545454546% significance.

Details:

- Using the composite log-likelihood ratio test, the significance of the inconsistency between datasets is 9.097690736410733 standard deviations.
- The number of sequences with data that is inconsistent is 0

```
-----
--- Comparing pass 1 to pass 4 (comparing 2 contexts) ---
-----
```

The datasets are INCONSISTENT at 0.4545454545454546% significance.

Details:

- Using the composite log-likelihood ratio test, the significance of the inconsistency between datasets is 20.14574482553519 standard deviations.
- The number of sequences with data that is inconsistent is 13
- The maximum SSTVD over all sequences is 0.41000000000000003
- The maximum SSTVD was observed for GxGxGx(Gx)<sup>256</sup>GxGxGx

```
-----
--- Comparing pass 1 to pass 5 (comparing 2 contexts) ---
-----
```

The datasets are INCONSISTENT at 0.4545454545454546% significance.

Details:

- Using the composite log-likelihood ratio test, the significance of the inconsistency between datasets is 34.10786497201147 standard deviations.
- The number of sequences with data that is inconsistent is 25
- The maximum SSTVD over all sequences is 0.54
- The maximum SSTVD was observed for GxGxGx(Gx)<sup>256</sup>GxGxGx

```
-----
--- Comparing pass 2 to pass 3 (comparing 2 contexts) ---
-----
```

Statistical hypothesis tests did NOT find inconsistency between the datasets at 0.4545454545454546% significance.

```
-----
--- Comparing pass 2 to pass 4 (comparing 2 contexts) ---
-----
```

The datasets are INCONSISTENT at 0.4545454545454546% significance.

Details:

- Using the composite log-likelihood ratio test, the significance of the inconsistency between datasets is 7.722146905324482 standard deviations.
- The number of sequences with data that is inconsistent is 1
- The maximum SSTVD over all sequences is 0.2799999999999997
- The maximum SSTVD was observed for GxGx(Gy)<sup>256</sup>GxGx

```
-----
--- Comparing pass 2 to pass 5 (comparing 2 contexts) ---
-----
```

The datasets are INCONSISTENT at 0.4545454545454546% significance.

Details:

- Using the composite log-likelihood ratio test, the significance of the inconsistency between datasets is 19.063124514167576 standard deviations.
- The number of sequences with data that is inconsistent is 14
- The maximum SSTVD over all sequences is 0.49
- The maximum SSTVD was observed for Gx(Gx)<sup>256</sup>GxGxGx

```
-----
--- Comparing pass 3 to pass 4 (comparing 2 contexts) ---
-----
```

Statistical hypothesis tests did NOT find inconsistency between the datasets at 0.4545454545454546% significance.

```
-----
--- Comparing pass 3 to pass 5 (comparing 2 contexts) ---
-----
```

The datasets are INCONSISTENT at 0.4545454545454546% significance.

Details:

- Using the composite log-likelihood ratio test, the significance of the inconsistency between datasets is 10.213028927361437 standard deviations.
- The number of sequences with data that is inconsistent is 3
- The maximum SSTVD over all sequences is 0.42000000000000004

- The maximum SSTVD was observed for  $Gx(Gx)^{256}GxGxGx$

-----  
 --- Comparing pass 4 to pass 5 (comparing 2 contexts) ---  
 -----

Statistical hypothesis tests did NOT find inconsistency between the datasets at 0.4545454545454546% significance.

```
In [14]: #Post-process the data, sorting the LLRs by sequence length
gate_sequence_gens = pygsti.construction.make_lsgst_lists(std1Q_XY.gates, fid
gate_sequence_family_dict = {}
for gate_seq in gate_sequences:
    generation = 0
    while gate_seq not in gate_sequence_gens[generation]:
        generation += 1
    gate_sequence_family_dict[gate_seq] = 2**generation
```

```
In [15]: pseudo_threshold = comparators_dict[0,4].get_LLR_pseudothreshold()
```

## Plotting the results

```
In [24]: #Plot JSD vs core sequence length for the comparison between the gate set w
#and the gate set with  $4 \times 10^{-3}$  radians of additional over rotation
plt.plot([gate_sequence_family_dict[gate_seq] for gate_seq in gate_sequences
plt.axhline(pseudo_threshold/(2*N), linestyle='--')
plt.xlabel('Core sequence length')
plt.ylabel('Jensen-Shannon Divergence')
```

```
Out[24]: Text(0,0.5, 'Jensen-Shannon Divergence')
```

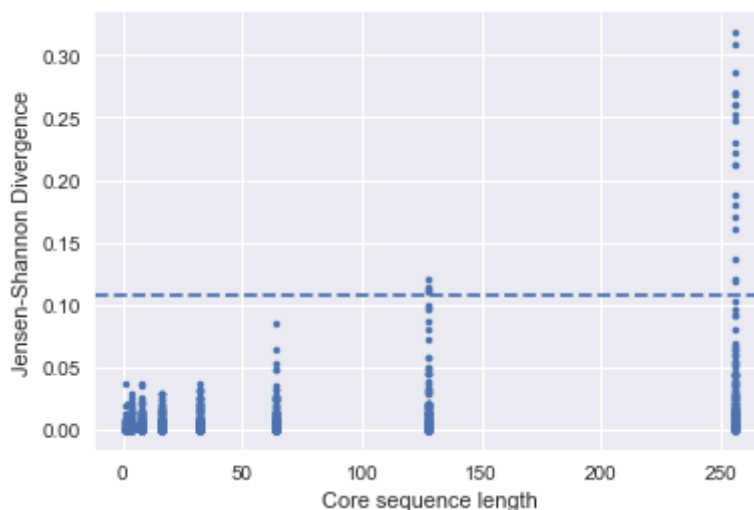

```
In [40]: #Now let's break down the above LLRs by whether or not the sequence's germ c
#an X-pi/2 gate, a Y-pi/2 gate, or a combination of X- and Y-pi/2 gates.
```

```
In [36]: germs
```

```
Out[36]: [GateString(Gx),  
          GateString(Gy),  
          GateString(GxGy),  
          GateString(GxGxGy),  
          GateString(GxGyGy),  
          GateString(GxGxGyGxGyGy)]
```

```
In [37]: x_only_germs = germs[:1]  
        y_only_germs = germs[1:2]  
        other_germs = germs[2:]  
  
        x_seqs = pygsti.construction.make_lsgst_experiment_list(std1Q_XY.gates, fiduc  
        y_seqs = pygsti.construction.make_lsgst_experiment_list(std1Q_XY.gates, fiduc  
        other_seqs = pygsti.construction.make_lsgst_experiment_list(std1Q_XY.gates, f
```

```

In [44]: plt.plot([gate_sequence_family_dict[gate_seq] for gate_seq in x_seqs],
                 [comparators_dict[0,4].llrs[gate_seq]/(2*N) for gate_seq in x_seqs],
                 'b', marker='v')
plt.axhline(pseudo_threshold/(2*N), linestyle='--')
plt.legend()
plt.xlabel('Core sequence length')
plt.ylabel('Jensen-Shannon Divergence')
plt.xscale('log')
plt.show()

plt.plot([gate_sequence_family_dict[gate_seq] for gate_seq in y_seqs],
         [comparators_dict[0,4].llrs[gate_seq]/(2*N) for gate_seq in y_seqs],
         'b', marker='v')
plt.axhline(pseudo_threshold/(2*N), linestyle='--')
plt.legend()
plt.xlabel('Core sequence length')
plt.ylabel('Jensen-Shannon Divergence')
plt.xscale('log')
plt.show()

plt.plot([gate_sequence_family_dict[gate_seq] for gate_seq in other_seqs],
         [comparators_dict[0,4].llrs[gate_seq]/(2*N) for gate_seq in other_seqs],
         'b', marker='v')
plt.axhline(pseudo_threshold/(2*N), linestyle='--')
plt.legend()
plt.xlabel('Core sequence length')
plt.ylabel('Jensen-Shannon Divergence')
plt.xscale('log')
plt.show()

```

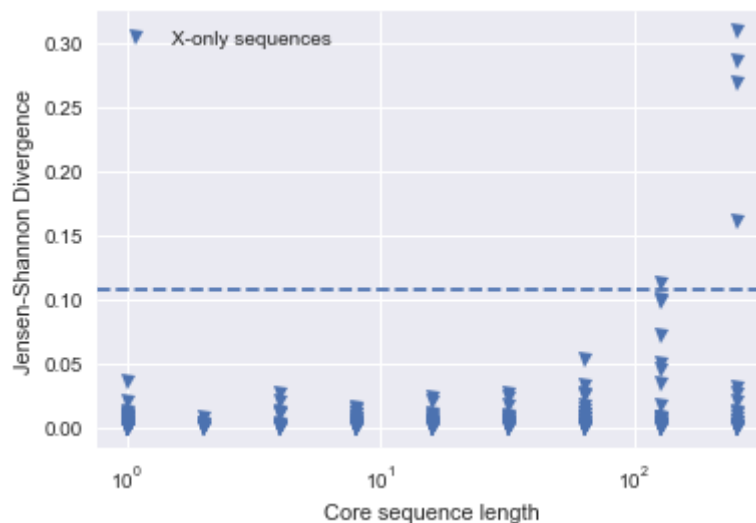



Fig2

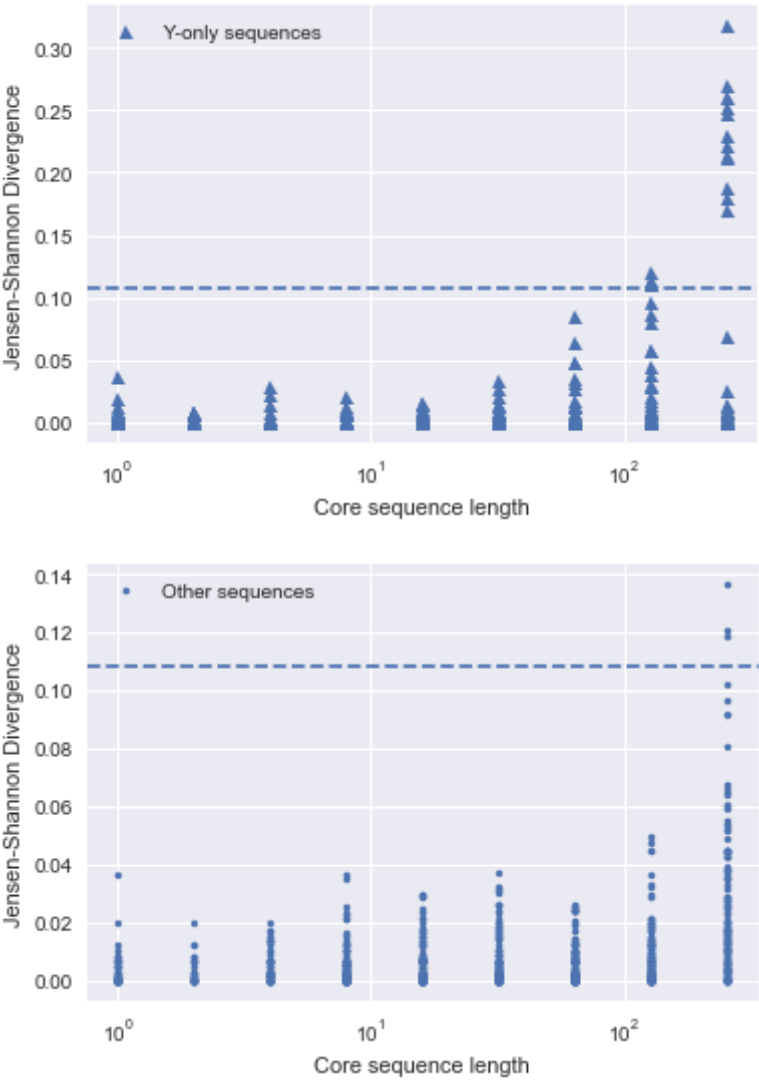

```

In [43]: #We can also visualize this data in another way.
#Each pixel corresponds to a gate sequence; it is shaded according to its LI
#Note that some circuits show up as multiple pixels in a plot.  Mouse over a
#"value" refers to log-likelihood ratio.

w = pygsti.report.Workspace()
w.init_notebook_mode(connected=False, autodisplay=True)

gssList = pygsti.construction.make_lsgst_structs(['Gx', 'Gy'], fiducials, fiducials)

w.ColorBoxPlot('dscmp', gssList[-1], None, None, dscomparator=comparators_default)

```

**Notebook Initialization Complete (+MathJax)**

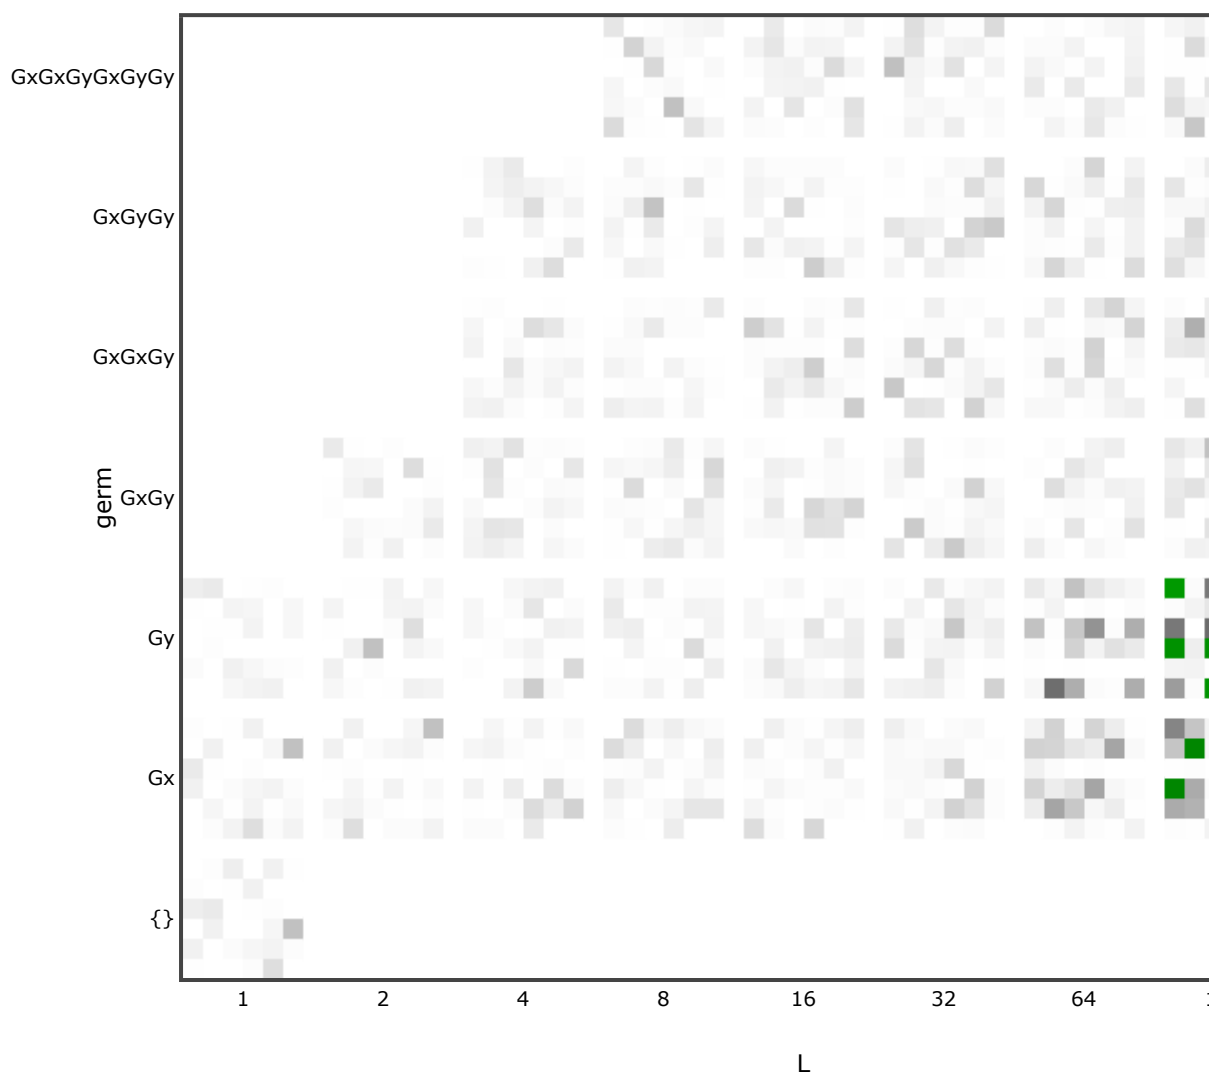

Out[43]: <pygsti.report.workspaceplots.ColorBoxPlot at 0x10ebe50f0>

In [ ]:
