# Supplementary material for: Probing context-dependent errors in quantum processors
Source: arXiv:1810.05651 ancillary file (2018-10-12)
Supplement: Supplementary file 2 [file Fig3.ipynb.pdf]

```
In [1]: #Import the relevant packages
import pygsti
import numpy as np
%matplotlib inline
from matplotlib import pyplot as plt
import seaborn
seaborn.set()
#import pygsti.extras
```

```
/Users/kmrudin/pyGSTi/packages/pygsti/tools/matrixtools.py:23: UserWarning: Could not import Cython extension - falling back to slower pure-python routines
  warnings.warn("Could not import Cython extension - falling back to slower pure-python routines")
```

## Getting the data

```
In [2]: #Declare the directed connectivity for ibmqx3. Qubit pairs are listed in (source, target)
directed_edge_list = [(0,1),(3,14),(13,4),(12,5),(6,11),(7,10),(9,8)]

#Declare horizontal distances from spectator qubit to edges driven by CNOTs
#Note that "-1" indicates a distance of 1 to the left.
distances = [-1,1,2,3,4,5,6]
```

```
In [3]: edge_to_distance_dict = {i[0]:i[1] for i in zip(directed_edge_list,distances)}
distance_to_edge_dict = {i[1]:i[0] for i in zip(directed_edge_list,distances)}
```

```
In [4]: data_dict = {}
```

```
In [5]: cases = ['before', 'during', 'after']
```

```
In [6]: path = 'IBM_data/'
```

```
In [7]: #a=0 # Spectator qubit is always 15
        for distance in distance_to_edge_dict:
            print (distance)
            b = distance_to_edge_dict[distance][0]#Define control qubit.
            c = distance_to_edge_dict[distance][1]#Define target qubit.
            for case in cases:
                # ds a is 15, b is 0, c is 1 after driving a.txt
                # print(path+'ds a is 15, b is '+str(b)+' , c is '+str(c)+' '+case+' c
                ds = pygsti.io.load_dataset(path+'ds a is 15, b is '+str(b)+' , c is
                data_dict[distance,case] = ds
```

-1

Loading from cache file: IBM\_data/ds a is 15, b is 0, c is 1 before driving a.txt.cache

Loading from cache file: IBM\_data/ds a is 15, b is 0, c is 1 during driving a.txt.cache

Loading from cache file: IBM\_data/ds a is 15, b is 0, c is 1 after driving a.txt.cache

1

Loading from cache file: IBM\_data/ds a is 15, b is 3, c is 14 before driving a.txt.cache

Loading from cache file: IBM\_data/ds a is 15, b is 3, c is 14 during driving a.txt.cache

Loading from cache file: IBM\_data/ds a is 15, b is 3, c is 14 after driving a.txt.cache

2

Loading from cache file: IBM\_data/ds a is 15, b is 13, c is 4 before driving a.txt.cache

Loading from cache file: IBM\_data/ds a is 15, b is 13, c is 4 during driving a.txt.cache

Loading from cache file: IBM\_data/ds a is 15, b is 13, c is 4 after driving a.txt.cache

3

Loading from cache file: IBM\_data/ds a is 15, b is 12, c is 5 before driving a.txt.cache

Loading from cache file: IBM\_data/ds a is 15, b is 12, c is 5 during driving a.txt.cache

Loading from cache file: IBM\_data/ds a is 15, b is 12, c is 5 after driving a.txt.cache

4

Loading from cache file: IBM\_data/ds a is 15, b is 6, c is 11 before driving a.txt.cache

Loading from cache file: IBM\_data/ds a is 15, b is 6, c is 11 during driving a.txt.cache

Loading from cache file: IBM\_data/ds a is 15, b is 6, c is 11 after driving a.txt.cache

5

Loading from cache file: IBM\_data/ds a is 15, b is 7, c is 10 before driving a.txt.cache

Loading from cache file: IBM\_data/ds a is 15, b is 7, c is 10 during driving a.txt.cache

Loading from cache file: IBM\_data/ds a is 15, b is 7, c is 10 after driving a.txt.cache

6

Loading from cache file: IBM\_data/ds a is 15, b is 9, c is 8 before driving a.txt.cache

Loading from cache file: IBM\_data/ds a is 15, b is 9, c is 8 during driving a.txt.cache

Loading from cache file: IBM\_data/ds a is 15, b is 9, c is 8 after driving a.txt.cache

```
In [8]: case_pairs = [('before', 'after'), ('before', 'during')]
```

```
In [9]: preps = pygsti.io.load_gatestring_list(path+'/4HS_prepFiducials.txt')
effects = pygsti.io.load_gatestring_list(path+'/4HS_measFiducials.txt')
```

```
In [10]: #The circuits in an LGST experiment are identical to the circuits in an LSGS
#if the germs are just the bare gates, and only L=1 is used.
germs=[pygsti.objects.GateString(('Gi',)), pygsti.objects.GateString(('Gh',))]
```

```
In [11]: lengths = [1]
```

```
In [12]: gatestrings = pygsti.construction.make_lsgst_experiment_list(['Gi', 'Gh', 'Gs'])
```

```
In [13]: num_strs = len(gatestrings)
```

## Analyzing the data

```
In [14]: comparators = {}
```

```
In [15]: corrected_significance_level = 1 - pygsti.tools.bonferroni_correction(0.95, 1)
print(corrected_significance_level)
```

```
0.0035714285714285587
```

```
In [16]: for distance in distances:
        for case0,case1 in case_pairs:
            print('\n')
            if (case0, case1) == ('before','after'):
                print('Distance to CNOT =',str(distance)+"", '('+str(case0)+'',
            else:
                print('Distance to CNOT =',str(distance)+"", '('+str(case0)+'',
            comparators[distance,case0,case1] = pygsti.objects.DataComparator([c
            comparators[distance,case0,case1].implement(significance=corrected_s
#         comparators[distance,case0,case1].compute_stat_sig_TVDs(verbosity=1
```

Distance to CNOT = -1. (before, after): checking for drift.  
Statistical hypothesis tests did NOT find inconsistency between the datasets at 0.3571428571428559% significance.

Distance to CNOT = -1. (before, during): checking for crosstalk.  
The datasets are INCONSISTENT at 0.3571428571428559% significance.

Details:

- Using the composite log-likelihood ratio test, the significance of the inconsistency between datasets is 20.861210808109302 standard deviations.
- The number of sequences with data that is inconsistent is 5
- The maximum SSTVD over all sequences is 0.08203125
- The maximum SSTVD was observed for GhGsGs(Gs)GhGsGh

Distance to CNOT = 1. (before, after): checking for drift.  
Statistical hypothesis tests did NOT find inconsistency between the datasets at 0.3571428571428559% significance.

Distance to CNOT = 1. (before, during): checking for crosstalk.  
The datasets are INCONSISTENT at 0.3571428571428559% significance.

Details:

- Using the composite log-likelihood ratio test, the significance of the inconsistency between datasets is 224.3417922858221 standard deviations.
- The number of sequences with data that is inconsistent is 20
- The maximum SSTVD over all sequences is 0.27734375
- The maximum SSTVD was observed for GhGsGs(Gs)GsGh

Distance to CNOT = 2. (before, after): checking for drift.  
Statistical hypothesis tests did NOT find inconsistency between the datasets at 0.3571428571428559% significance.

Distance to CNOT = 2. (before, during): checking for crosstalk.

The datasets are INCONSISTENT at 0.3571428571428559% significance.

Details:

- Using the composite log-likelihood ratio test, the significance of the inconsistency between datasets is 42.72203701931253 standard deviations.
- The number of sequences with data that is inconsistent is 11
- The maximum SSTVD over all sequences is 0.1298828125
- The maximum SSTVD was observed for GhGsGs(Gi)GhGsGh

Distance to CNOT = 3. (before, after): checking for drift.

Statistical hypothesis tests did NOT find inconsistency between the datasets at 0.3571428571428559% significance.

Distance to CNOT = 3. (before, during): checking for crosstalk.

The datasets are INCONSISTENT at 0.3571428571428559% significance.

Details:

- Using the composite log-likelihood ratio test, the significance of the inconsistency between datasets is 15.62134059274328 standard deviations.
- The number of sequences with data that is inconsistent is 3
- The maximum SSTVD over all sequences is 0.056640625
- The maximum SSTVD was observed for GhGs(Gi)GsGh

Distance to CNOT = 4. (before, after): checking for drift.

Statistical hypothesis tests did NOT find inconsistency between the datasets at 0.3571428571428559% significance.

Distance to CNOT = 4. (before, during): checking for crosstalk.

The datasets are INCONSISTENT at 0.3571428571428559% significance.

Details:

- Using the composite log-likelihood ratio test, the significance of the inconsistency between datasets is 7.813514758727584 standard deviations.
- The number of sequences with data that is inconsistent is 2
- The maximum SSTVD over all sequences is 0.029296875
- The maximum SSTVD was observed for GhGsGs(Gs)GsGh

Distance to CNOT = 5. (before, after): checking for drift.

Statistical hypothesis tests did NOT find inconsistency between the datasets at 0.3571428571428559% significance.

Distance to CNOT = 5. (before, during): checking for crosstalk.

The datasets are INCONSISTENT at 0.3571428571428559% significance.

Details:

- Using the composite log-likelihood ratio test, the significance of the inconsistency between datasets is 9.054125539110192 standard deviation s.
- The number of sequences with data that is inconsistent is 2
- The maximum SSTVD over all sequences is 0.029296875
- The maximum SSTVD was observed for GhGs(Gi)GhGsGh

Distance to CNOT = 6. (before, after): checking for drift.

Statistical hypothesis tests did NOT find inconsistency between the datasets at 0.3571428571428559% significance.

Distance to CNOT = 6. (before, during): checking for crosstalk.

The datasets are INCONSISTENT at 0.3571428571428559% significance.

Details:

- Using the composite log-likelihood ratio test, the significance of the inconsistency between datasets is 9.85336671272647 standard deviations.
- The number of sequences with data that is inconsistent is 2
- The maximum SSTVD over all sequences is 0.0234375
- The maximum SSTVD was observed for GhGs(Gi)GhGsGh

```
In [17]: #Data for Fig. 3
case0 = 'before'
case1 = 'during'
print('Distance\t SSTVD\t\t Gatestring\t\t Gatestring length')
for distance in distances:
#     maxidx = np.argmax(np.array(list(comparators[distance,case0,case1].sstvds.values())))
#     sequence, max_sstv = comparators[distance,case0,case1].get_maximum_SSTVD(sequence)
    print(distance, '\t\t', max_sstv, '\t\t', sequence, '\t\t', len(sequence))
#     print(distance, '\t\t', comparators[distance,case0,case1].sstvds[sequence])
#     np.max(np.array(list(comparators[distance,case0,case1].sstvds.values())))
```

| Distance | SSTVD        | Gatestring         | Gatestring length |
|----------|--------------|--------------------|-------------------|
| -1       | 0.08203125   | GhGsGs (Gs) GhGsGh | 7                 |
| 1        | 0.27734375   | GhGsGs (Gs) GsGh   | 6                 |
| 2        | 0.1298828125 | GhGsGs (Gi) GhGsGh | 7                 |
| 3        | 0.056640625  | GhGs (Gi) GsGh     | 5                 |
| 4        | 0.029296875  | GhGsGs (Gs) GsGh   | 6                 |
| 5        | 0.029296875  | GhGs (Gi) GhGsGh   | 6                 |
| 6        | 0.0234375    | GhGs (Gi) GhGsGh   | 6                 |

```
In [18]: [comparators[distance,case0,case1].get_maximum_SSTVD()[1] for distance in distances]
```

```
Out[18]: [0.08203125,
0.27734375,
0.1298828125,
0.056640625,
0.029296875,
0.029296875,
0.0234375]
```

## Plotting the results

```
In [19]: plt.plot(distances,[comparators[distance,case0,case1].get_maximum_SSTVD()[1]  
plt.xlabel('Distance')  
plt.ylabel('SSTVD')
```

```
Out[19]: Text(0,0.5,'SSTVD')
```

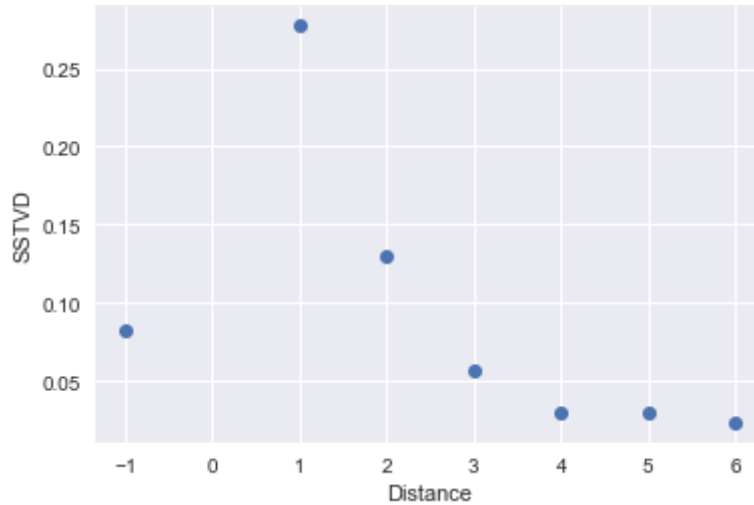

```
In [20]: #Additional data analysis visualization may be performed.  
#Here is a small sampling.
```

```
In [21]: w = pygsti.report.Workspace()  
w.init_notebook_mode(connected=False, autodisplay=True)
```

**Notebook Initialization Complete (+MathJax)**

```
In [22]: #Plot p-value histograms for each of the (driving-no-)
for distance in distances:
    print('distance='+str(distance))
    w.DatasetComparisonHistogramPlot(comparators[distance, 'before', 'during']
```

distance=-1

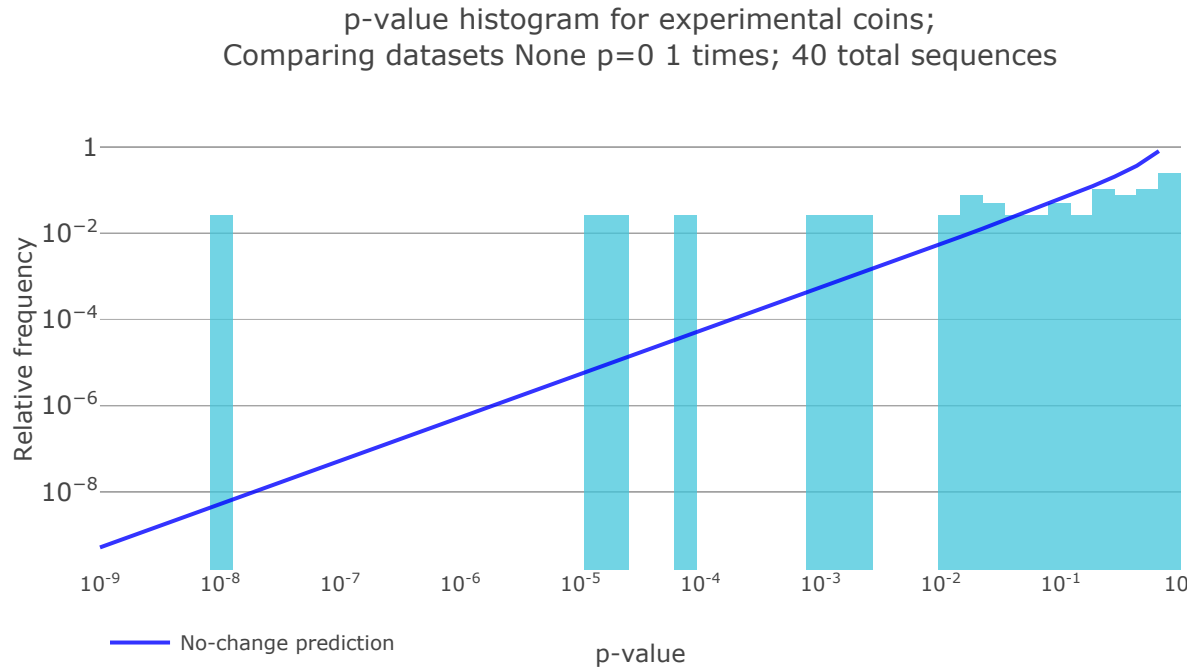

distance=1

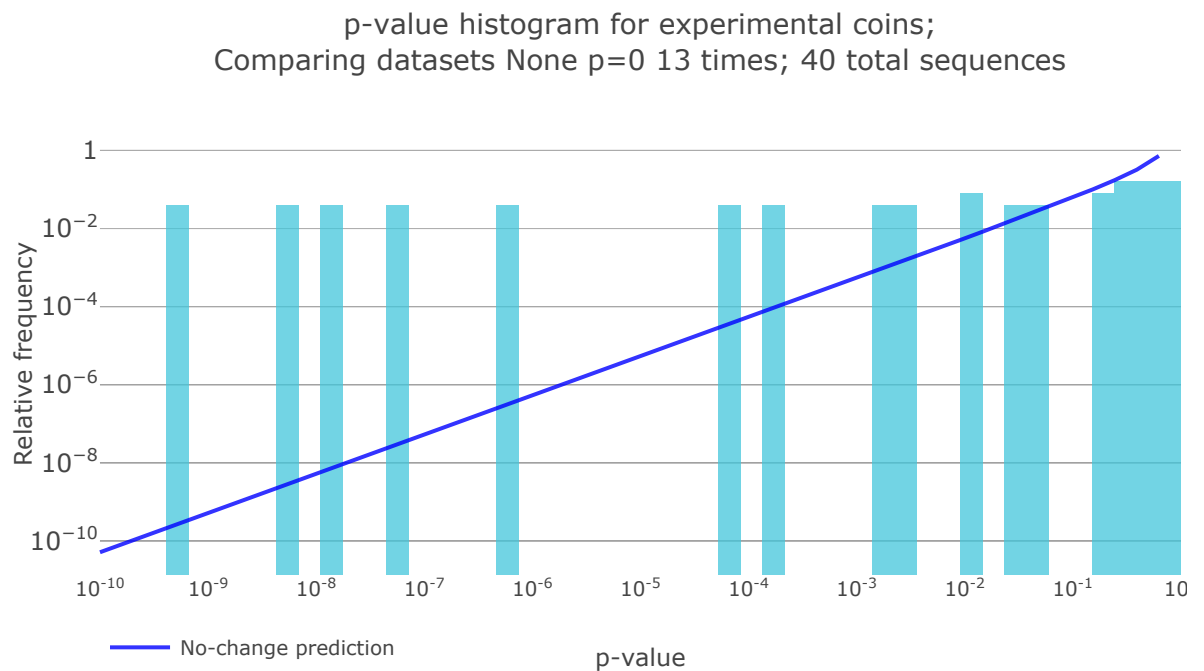



distance=2

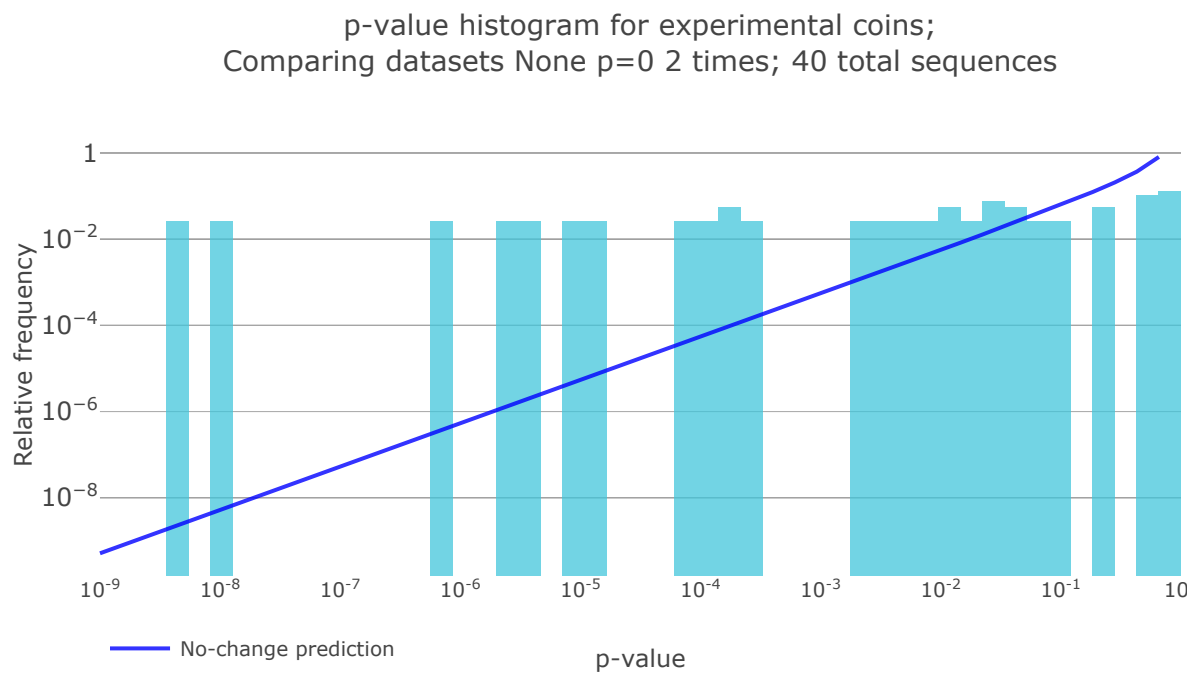

distance=3

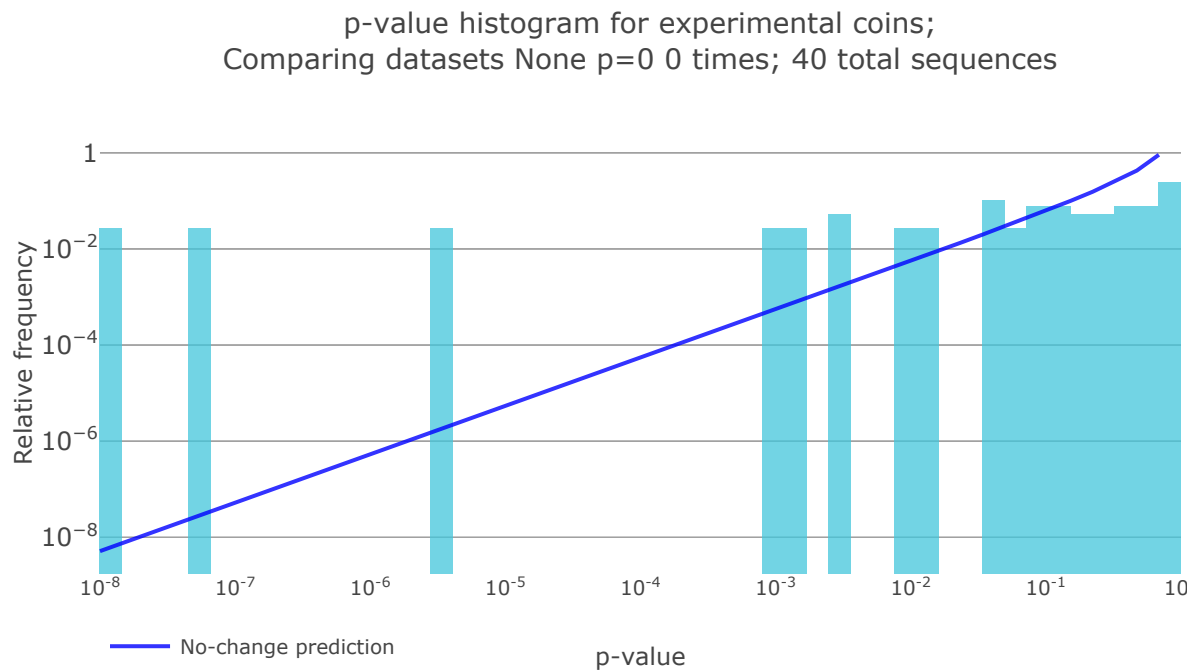

distance=4

p-value histogram for experimental coins;  
Comparing datasets None p=0 0 times; 40 total sequences

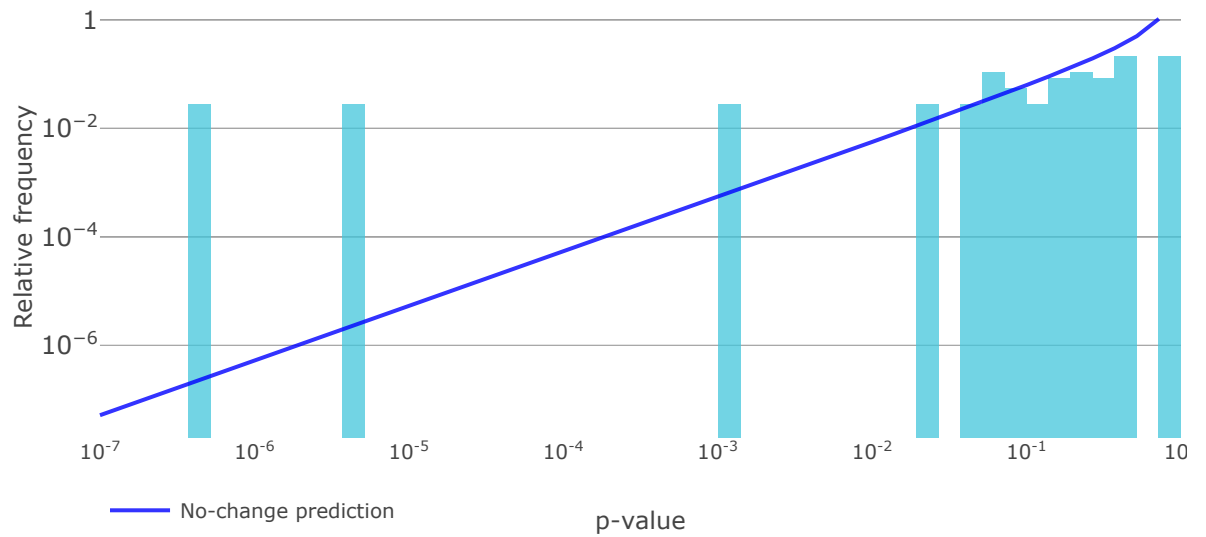

distance=5

p-value histogram for experimental coins;  
Comparing datasets None p=0 0 times; 40 total sequences

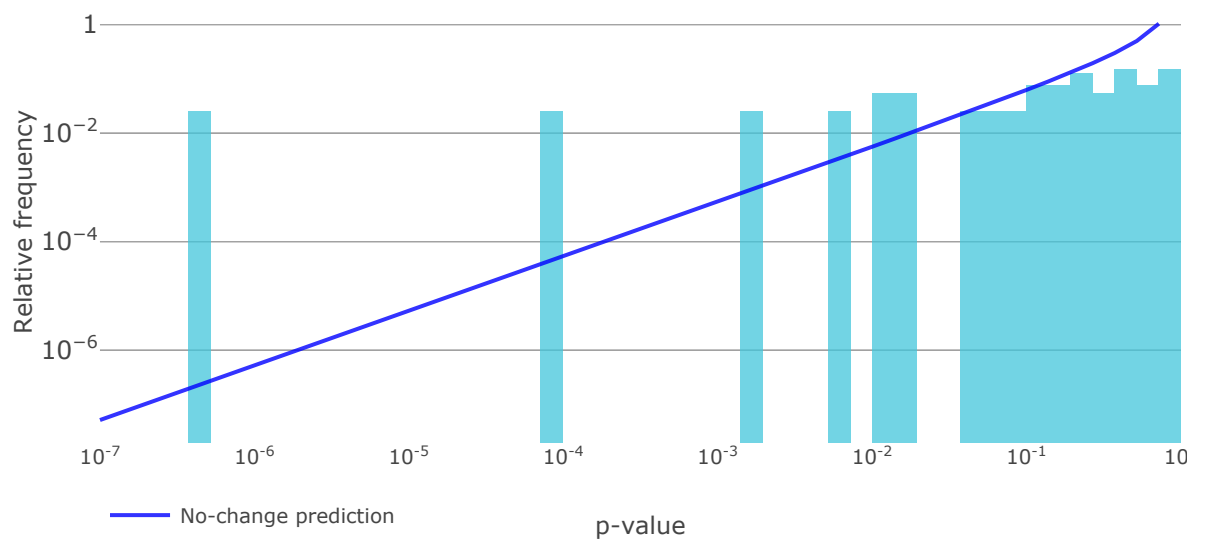

distance=6

p-value histogram for experimental coins;  
Comparing datasets None p=0 0 times; 40 total sequences

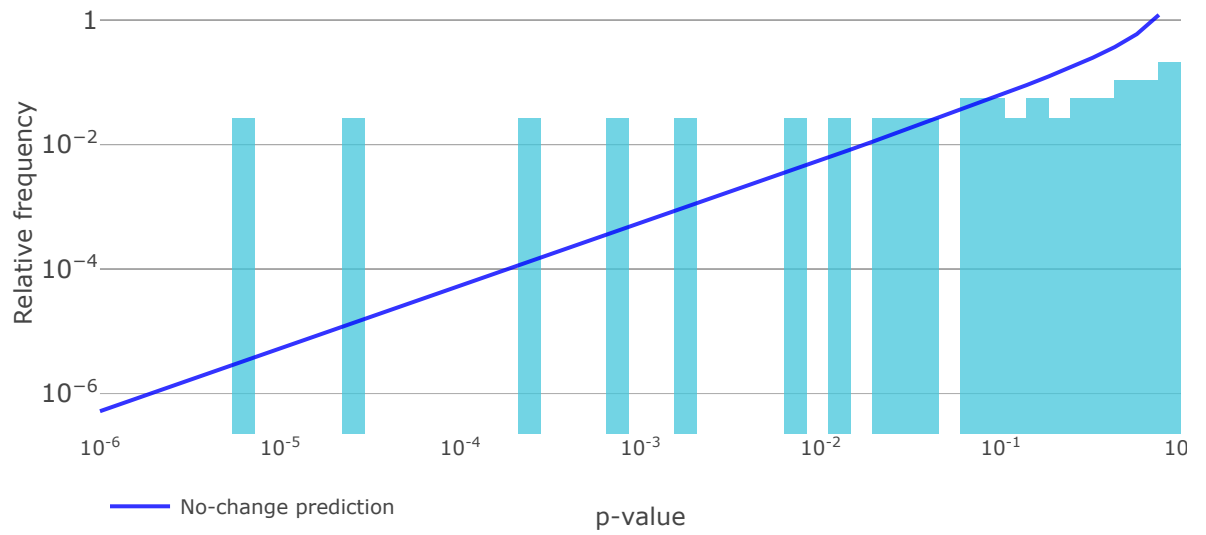

```
In [23]: gssList = pygsti.construction.make_lsgst_structs(['Gi', 'Gh', 'Gs'], preps, ef
```

```
In [24]: #See which specific circuits detect the crosstalk.
#Note that some circuits show up as multiple pixels in a plot.  Mouse over p
#"value" refers to log-likelihood ratio.
for distance in distances:
    print('distance='+str(distance))
    w.ColorBoxPlot('dscmp', gssList[-1], None, None, dscomparator=comparator
```

distance=-1

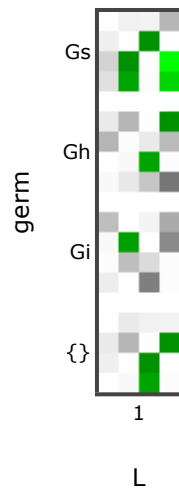

distance=1

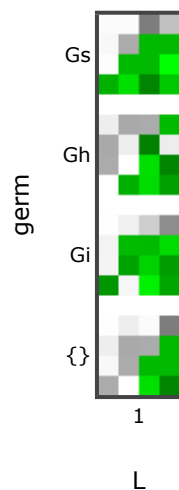

distance=2

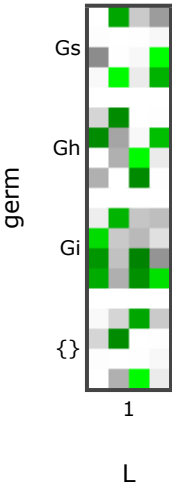

distance=3

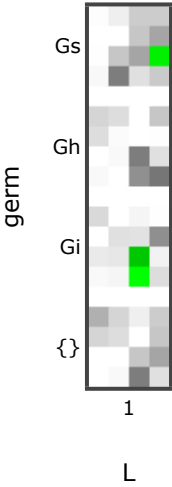

distance=4

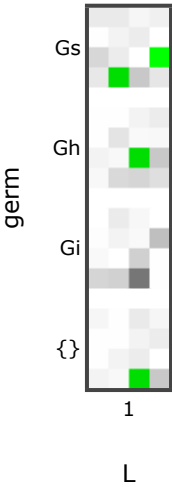

distance=5

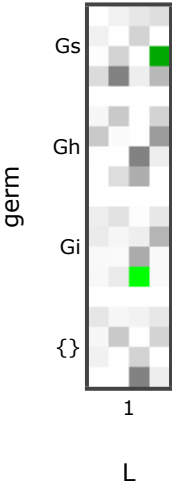

distance=6

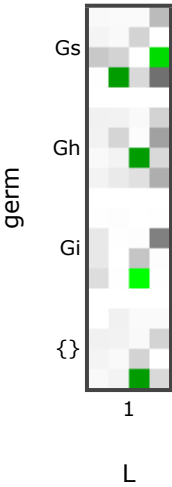

```
In [ ]:
```
